# Supplementary material for: Latent Multimodal Functional Graphical Model Estimation
Source: arXiv:2210.17237 source file (2023-10-01)
Supplement: Supplementary file 1 [file 3_proof_3.tex]

\subsection{Proofs of Lemma~\ref{lemma:graddiff_A} and Lemma~\ref{lemma:graddiff_B}} \label{ssec:edge_auxlemma_3}

We
\begin{proof}[Proof of Lemma~\ref{lemma:graddiff_A}]
For notation simplicity, we define $\Mscr_i={\eNi\cup\{i\}}$ for $\pseq$ and write
\begin{align*}
    \norm{
        \nabla_{\Amk}f_{\hat\Yb}(\setAk,\setBk)
        &-
        \nabla_{\Amk}f(\setAk,\setBk)
    }_F^2\\
    &=
    \norml{
    \sum_{j=1}^p(\eb_j^\top\otimes \Ib_k)\cbr{\sum_{i=1}^p\tBikT \tBik (\Ib_p\otimes \Amk )(\hsCov-\sCov)}(\eb_j\otimes \Ib_{k_m})
    }_F^2\\
    &\leq p
    \sum_{i=1}^p|\Mscr_i|^2
    \norml{
    \tBikfreeT{\Mscr_i}
    \tBikfree{\Mscr_i}  
    \bigAs{|\Mscr_i|}{\Amk}
    (\hsCovfree{\Mscr_i}{\Mscr_i}
    -
    \sCovfree{\Mscr_i}{\Mscr_i})
    }_F^2.\\
    \intertext{Recall that $|\Mscr_i|=|\eNi\cup\{i\}|\leq \gamma_1(s^{\star}+1)/2$ and we can bound the above display as}
    &\leq
    \frac{\gamma_1^2(s^{\star}+1)^2p}{4}
    \sum_{i=1}^p(1+C_A)^2(1+C_B)^4\norm{\pAmk}_2^2\norm{\pBik}_F^4
    \norm{\hsCovfree{\Mscr_i}{\Mscr_i}
    -
    \sCovfree{\Mscr_i}{\Mscr_i}
    }_2^2.
\end{align*}
We can write the last term of the above equation as
\begin{align*}
    \norm{\hsCovfree{\Mscr_i}{\Mscr_i}
    -
    \sCovfree{\Mscr_i}{\Mscr_i}
    }_2
    &\leq 
    \norml{
        \hsCovfree{\Mscr_i}{\Mscr_i}
        -
        \EE\rbr{
            \hsCovfree{\Mscr_i}{\Mscr_i}
        }
    }_2\\
    &\quad+
        \norml{
        \sCovfree{\Mscr_i}{\Mscr_i}
        -
        \EE\rbr{
            \sCovfree{\Mscr_i}{\Mscr_i}
        }
    }_2\\
    &\quad+
        \norml{
        \EE\rbr{
            \hsCovfree{\Mscr_i}{\Mscr_i}
        }
        -
        \EE\rbr{
            \sCovfree{\Mscr_i}{\Mscr_i}
        }
    }_2\\
    &\leq \Ical_{31,m}+ \Ical_{32,m} +\Ical_{33,m}.
\end{align*}
First, by Cauchy-interlacing therem, we have 
\begin{equation}\label{eq:equality}
\norml{\EE\rbr{
        \hsCovfree{\Mscr_i}{\Mscr_i}
    }}_2
\leq 
\max_{i\in\Mscr_i}
\norml{
\EE\rbr{
        \hsCovfree{i}{i}
    }
}
\leq
\max_{i\in\Mscr_i}
\norm{\Kscr_{m,i}}
\leq
\max_{i\in\Mscr_i}
\norml{\EE\rbr{\sCovfree{i}{i}}}
\leq 
\rho_x.
\end{equation}
Then, since $N\gtrsim\max_{\mseq} 
k_m(s^\star+1)
+\log M + \log p
$, we can apply Lemma~\ref{lemma:ci} and obtain
\begin{align*}
    \Ical_{31,m}=\norml{
        \hsCovfree{\Mscr_i}{\Mscr_i}
        -
        \EE\rbr{
            \hsCovfree{\Mscr_i}{\Mscr_i}
        }
    }_2\leq C_0\rho_x\sqrt{\frac{k_m(s^\star+1)+\log M+ \log p}{N}},
\end{align*}
and
\begin{align*}
        \Ical_{32,m}=\norml{
        \sCovfree{\Mscr_i}{\Mscr_i}
        -
        \EE\rbr{
            \sCovfree{\Mscr_i}{\Mscr_i}
        }
    }_2\leq C_0'\rho_x\sqrt{\frac{k_m(s^\star+1)+\log M+ \log p}{N}},
\end{align*}
with probability at least $1-(pM)^{-1}2\exp\{-k_m(s^\star+1)\}$.

Recall the definition of $\zeta_m^{k_m}$ defined in~\eqref{eq:defzeta}. Since $\SCfive$, Lemma~\ref{lemma:Kscr_sample bound} tells us that 
$$
\norm{
\hat\Kscr_{\bar m}
-
\Kscr_{\bar m}
}\leq \hsnorm{\hat\Kscr_{\bar m}
-
\Kscr_{\bar m}}\leq \zeta_m^{k_m},
$$ 
probability at least $1-(pM)^{-1}\delta_1$. Then, we can apply Lemma~\ref{lemma:perturbation_bound} to bound $\Ical_{33,m}$ and plug in $\norm{
\hat\Kscr_{\bar m}
-
\Kscr_{\bar m}
}^2\lesssim N^{-1}(-\log\delta_1+\log P + \log M)$ by Lemma~\ref{lemma:Kscr_sample bound} 
\begin{align*}
    (\Ical_{33,m})^2
    =
    C_0\rho_x 
    \frac{
        k_m\{\log pM+\log(1/\delta_1)\}
    }{
        (\zeta_m^{k_m})^2N
    }\norml{\sum_{j\in\Mscr_i}\Kscr_{m,j}}.
\end{align*}
Combining the results of $\Ical_{31,m}$,$\Ical_{32,m}$,$\Ical_{33,m}$ and taking the union bound over $\pseq$, we can obtain that
\begin{multline*}
    \norm{
        \nabla_{\Amk}f_{\hat\Yb}(\setAk,\setBk)
        -
        \nabla_{\Amk}f(\setAk,\setBk)
    }_F^2
    \leq 
   \Upsilon_{10}p^2(s^\star+1)^2
    \frac{k_m(s^\star+1)\vee k_m(\log M + \log p+\log1/\delta_1)}{N},
\end{multline*}
with probability at least $1-2M^{-1}\exp\{-k_m(s^\star+1)\}-M^{-1}\delta_1$.
\end{proof}
\marginnote{Discuss this: $\dotp{e_j}{\hat e_j}\geq 0$ for $j\in\NN$.
We need to add a "sign" operator in the metric so that this would always hold. It seems like we will always have it.

}

\begin{proof}[Proof of Lemma~\ref{lemma:graddiff_B}]
Recall the definitions of $\bar\Scal_i$ in~\eqref{eq:defsupport} and $\eNi,\barNi$ defined in~\eqref{eq:defneighbour}. Write
\begin{align*}
    \norm{
        [\nabla_{\Bik}f_{\hat\Yb}&(\setAk,\setBk)
        -
        \nabla_{\Bik}f(\setAk,\setBk)]_{\bar\Scal_i}
    }_F^2\\
    &\leq 
    M\sum_{m=1}^M
    \norml{
        \tBikfree{\eNi\cup\{i\}} \bigAs{|\eNi\cup\{i\}|}{\Amk}
        \rbr{
        \hsCovfree{\eNi\cup\{i\}}{\barNi}
        -
        \sCovfree{\eNi\cup\{i\}}{\barNi}
        }
        \bigAs{|\barNi|}{\Amk}^2
    }_F^2\\
    &\leq 
    M\sum_{m=1}^M\norm{\Amk}_2^4\norm{\tBik}_F^2
    \norml{
    \hsCovfree{\eNi\cup\{i\}}{\barNi}
        -
    \sCovfree{\eNi\cup\{i\}}{\barNi}
        }_2^2\\
    &\leq M\sum_{m=1}^M(1+C_A)^4(1+C_B)^2\norm{\pAmk}_2^4\norm{\ptBik}_F^2\norml{
    \hsCovfree{\eNi\cup\{i\}}{\barNi}
        -
    \sCovfree{\eNi\cup\{i\}}{\barNi}
        }_2^2,
\end{align*}
where the last line follow by the assumption that
$\norm{\Amk-\pAmk}_2\leq C_A\norm{\pAmk}_2$
and 
$\norm{\tBik-\ptBik}_F^2=\norm{\Bik-\pBik}_F^2\leq C_B^2\norm{\pBik}_F^2$ for $\mseq$ and $\pseq$.

The upper bound for $\norm{
    \hsCovfree{\eNi\cup\{i\}}{\barNi}
        -
    \sCovfree{\eNi\cup\{i\}}{\barNi}
        }_2$ can be obtained in the same way as Lemma~\ref{lemma:graddiff_A} and hence omit for brevity. Consequently, we obtain
\begin{multline*}
    \norm{
        [\nabla_{\Bik}f_{\hat\Yb}(\setAk,\setBk)
        -
        \nabla_{\Bik}f(\setAk,\setBk)]_{\bar\Scal_i}
    }_F^2
    \leq \Upsilon_{10}M^2\max_{\mseq}
    \frac{k_m(s^\star+1)\vee k_m(\log M + \log p+\log1/\delta_1)}{N},
\end{multline*}
with probability at least $1-2\sum_{m=1}^M(pM)^{-1}\exp\{-k_m(s^\star+1)\}-\delta_1\geq 1 - 2p^{-1}\max_{\mseq}\exp\{-k_m(s^\star+1)\}-p^{-1}\delta_1$.
\end{proof}
