# Supplementary material for: Latent Multimodal Functional Graphical Model Estimation
Source: arXiv:2210.17237 source file (2023-10-01)
Supplement: Supplementary file 2 [file 4_initialization.tex]

\section{Initialization}

\subsection{Preliminaries}
\begin{proposition}\label{prop:Kzcompact}
$\Kscr_{z,i}$ is a compact operator for $\pseq$. 
\end{proposition}
This is a direct result from the fact that $\Kscr_{m,i}$ and $\Ascr_m$ for $\mseq$ and $\pseq$ are compact.
\begin{proof}[Proof of Proposition~\ref{prop:Kzcompact}]
We give a detailed proof here. Take $p=1$ and the generalization for $p>1$ follows similarly. For any $u,v\in\HH_z$ and $\mseq$, we have
\begin{align*}
    \Kscr_{z,1}(u,v) 
    &=
    \dotp{\Kscr_{z,1}u}{v}.\\
     \intertext{Apply Fubini's theorem, we can write the above line as}  
    &= \EE
    \dotp{\chi_{z,1}}{\cdot}
    \dotp{\chi_{z,1}}{u}\\
    &=\EE
    \dotp{\Ascr_m\chi_{m,1}}{v}
    \dotp{\chi_{m,1}}{\Ascr_m^*u}.\\
    \intertext{Apply Fubini's theorem once more, we can write the above line as}
    & = 
    \dotp{\Ascr_{m}\Kscr_{m,i}\Ascr_m^*u}{v}.
\end{align*}
Therefore, we can write $\Kscr_{z,1}=\Ascr_{m}\Kscr_{m,i}\Ascr_m^*$. Since $\Ascr_m$ is compact, it follows that $\Ascr_m^*$ is compact. Using the fact that the composite of compact operators is compact, we could conclude the proof. 
\end{proof}

\begin{proof}[Proof of Proposition~\ref{prop:R_property}]
Recall that $\Kscr_{mm',i}= \Kscr_{m,i}^{1/2}\Rscr_{mm',i}\Kscr_{m',i}^{1/2}$. Pre-multiply both sides by $\Ascr_{m}$ and post-multiply both sides by $\Ascr_m^*$, we could obtain
\[
\Ascr_{m}\Kscr_{mm',i}\Ascr_m^*
= 
\rbr{\Ascr_{m}\Kscr_{m,i}^{1/2}}\Rscr_{mm',i}\rbr{\Kscr_{m',i}^{1/2}\Ascr_m^*}.
\]
Since $\Ascr_{m}\Kscr_{mm',i}\Ascr_m^*=\Kscr_{z,i}$, we can write $\Rscr_{mm',i}= 
\rbr{\Ascr_{m}\Kscr_{m,i}^{1/2}}^{-1}
\Kscr_{z,i}\rbr{\Kscr_{m',i}^{1/2}\Ascr_{m'}^*}^{-1}$. Then, for any $g\in\overline{Im(\Kscr_{m',i}^{1/2}\Ascr_{m'}^*)}$, we have
\begin{align*}
\rbr{\Rscr_{mm',i}}^*\Rscr_{mm',i}g
&=
\rbr{\Ascr_{m'}\Kscr_{m',i}^{1/2}}^{-1}
\Kscr_{z,i}
\rbr{\Kscr_{m,i}^{1/2}\Ascr_{m}^*}^{-1}
\rbr{\Ascr_{m}\Kscr_{m,i}^{1/2}}^{-1}
\Kscr_{z,i}\rbr{\Kscr_{m',i}^{1/2}\Ascr_{m'}^*}^{-1}
g\\
&=\rbr{\Ascr_{m'}\Kscr_{m',i}^{1/2}}^{-1}
\Kscr_{z,i}\rbr{\Kscr_{m',i}^{1/2}\Ascr_{m'}^*}^{-1} g\\
&=g.
\end{align*}
The equality for $\Rscr_{mm',i}\rbr{\Rscr_{mm',i}}^*f=f$ for $f\in\overline{Im(\Kscr_m^{1/2}\Ascr_m^*)}$ follows similarly. From this result, we could observe that $\Rscr_{mm',i}^*\Rscr_{mm',i}$ acts as an identity operator on the domain $\overline{Im(\Kscr_{m',i}^{1/2}\Ascr_{m'}^*)}$. 

This implies that if $\Rscr_{mm',i}$ is compact and $1$ is an eigenvalue of $\Rscr_{mm',i}$, its multiplicity must be finite. Therefore, we could conclude that the rank of $\Kscr_{m',i}^{1/2}\Ascr_{m'}^*$ must be finite. The same statement also holds for $\Kscr_{m,i}^{1/2}\Ascr_{m}^*$. Since $\Kscr_{z,i}=\Ascr_m\Kscr_{m,i}^{1/2}\Kscr_{m,i}^{1/2}\Ascr_m^*$, it follows that the rank of $\Kscr_{z,i}$ is finite.
\end{proof}

Our analysis of functional CCA is based on~\citep{hsing2015theoretical}. However, since we use different notion of the inner product, it is worth verifying that some properties still hold under our setting.
\begin{lemma}\label{lemma:existence_c}
Given two Hilbert spaces $\GG(\Kscr_1)$ and $\GG(\Kscr_2)$ with $\Kscr_1 =\EE (\chi_1 \otimes \chi_1)$ and $\Kscr_2 = \EE(\chi_2 \otimes \chi_2)$,
there are operators $\Cscr_{12}\in\mathfrak{B}(\GG(\Kscr_2),\GG(\Kscr_1))$
and $\Cscr_{21}\in\mathfrak{B}(\GG(\Kscr_1),\GG(\Kscr_2))$ such that
\begin{align*}
    \Cov(\dotp{\chi_1}{f}\dotp{\chi_2}{g}) = \dotp{f}{\Cscr_{12}g}_{\GG(\Kscr_1)} = \dotp{\Cscr_{21}f}{g}_{\GG(\Kscr_2)},
\end{align*}
for $f\in\GG(\Kscr_1)$ and $g\in\GG(\Kscr_2)$. Furthermore, the operator norm $\norm{\Cscr_{12}}=\norm{\Cscr_{21}}\leq 1$.
\end{lemma}
\begin{proof}
Fix $g\in\GG(\Kscr_2)$, we define the functional:
\[
\ell_g(f) = \Cov(\dotp{\chi_1}{f}\dotp{\chi_2}{g}),
\]
which is linear because the covariance is bilinear. By Cauchy-Schwarz, we can proof the $\ell_g(f)$ is bounded:
\begin{align}
\abr{\ell_g(f)}^2\leq\Var({\dotp{\chi_1}{f}})\Var({\dotp{\chi_2}{g}})
&=\rbr{\sum_{j=1}^\infty \lambda_{1j}\rbr{\dotp{f}{e_{1j}}}^2}
\rbr{\sum_{j=1}^\infty \lambda_{2j}\rbr{\dotp{g}{e_{2j}}}^2}\notag\\
&=\norm{f}_{\GG(\Kscr_1)}^2\norm{g}_{\GG(\Kscr_2)}^2<\infty.\label{eq:lg_boundedness}
\end{align}
Since $\ell_g$ is linear and bounded, by the Riez-representation theorem, there exists an element $\Cscr_{12}g\in\GG(\Kscr_1)$ such that
\begin{equation}\label{eq:riez}
    \ell_g(f) = \dotp{f}{\Cscr_{12}g}_{\GG(\Kscr_1)}.
\end{equation}

Next, we want to verity that $\norm{\Cscr_{12}}\leq 1$. Write
\begin{align*}
    \norm{\Cscr_{12}g}_{\GG(\Kscr_1)}& = 
    \left\langle{
        \Cscr_{12}g},
        {\frac{\Cscr_{12}g}{\norm{\Cscr_{12}g}_{\GG(\Kscr_2)}}}
    \right\rangle_{\GG(\Kscr_2)}\\
    &\leq \sup_{\norm{f}_{\GG(\Kscr_1)=1}}\dotp{\Cscr_{12}g}{f}_{\GG({\Kscr_1})}\\
    &\leq \norm{g}_{\GG(\Kscr_2)},
\end{align*}
where the last line is followed by~\eqref{eq:lg_boundedness} and~\eqref{eq:riez}. Therefore, $\norm{\Cscr_{12}}\leq1$. We can construct $\Cscr_{21}$ in the similar way and hence omit the proof for brevity. 
\end{proof}
In the following, we will discuss the relation of $\Cscr_{12}$, $\Kscr_{1}$, $\Kscr_{2}$ and $\Kscr_{12}$.
\begin{lemma}\label{lemma:RC_svd}
Let $\Kscr_1:=\EE(\chi_1\otimes\chi_1)$ be the eigen system $\{(\lambda_{1,j},e_{1,j})\}_{j\in\NN}$ and $\Kscr_2:=\EE(\chi_2\otimes\chi_2)$ has the eigen system $\{(\lambda_{2,j},e_{2,j})\}_{j\in\NN}$ and define $\tilde{e}_{m,j}=\lambda_{m,j}^{1/2}e_{m,j}$ for $m=1,2$ and $j\in\NN$.
There exists a bounded operator $\Rscr_{12}\in\mathfrak{B}(\HH_2,\HH_1)$ with $\norm{\Rscr_{12}}\leq 1$ such that $\Kscr_{12}=\Kscr_1^{1/2}\Rscr_{12}\Kscr_{2}^{1/2}$. For  $i,j\in\NN$, we have
\begin{equation}\label{eq:RequalC}
\dotp{\tilde{e}_{1,i}}{\Cscr_{12}\tilde{e}_{2,j}}_{\GG_{\bar 1}}
=
\dotp{e_{1i}}{\Rscr_{12}e_{2j}}_{\HH_1}.
\end{equation}
Assume that both $\Cscr_{12}$ and $\Rscr_{12}$ are compact and let $\{(\rho_j,f_{1,j},f_{2,j})\}_{j\in\NN}$ be the singular system of $\Cscr_{12}$ and $\{(\check \rho_j,\check f_{1,j}, \check f_{2,j})\}_{j\in\NN}$ be the singular system of $\Rscr_{12}$. Then, for $j\in\NN$ and $m=1,2$, we have $\rho_j=\check\rho_j$ and
\begin{equation}\label{eq:RCsvd}
\check f_{m,j} = \sum_{i=1}^\infty
\dotp{f_{m,j}}{\tilde{e}_{m,i}}_{\GG_{m}}
e_{m,i},\quad
f_{m,j} = 
\sum_{i=1}^\infty
\dotp{\check{f}_{m,j}}{{e}_{m,i}}_{\HH_{m}}\tilde{e}_{m,i}.
\end{equation}
\end{lemma}
\begin{proof}
The existence of $\Rscr_{12}$ is justified by Theorem 7.2.10 in~\citep{hsing2015theoretical}. To show the first result, write
\begin{align*}
    \dotp{\tilde{e}_{1,i}}{\Cscr_{12}\tilde{e}_{2,j}}_{\GG_{ 1}} 
    = 
    \Cov(
        \dotp{\chi_1}{\tilde{e}_{1,i}}
        \dotp{\chi_2}{\tilde{e}_{2,j}}
    )
    &=
    \frac{
        \Cov(
        \dotp{\chi_1}{{e}_{1,i}}
        \dotp{\chi_2}{{e}_{2,j}}
    )
    }{\lambda_{1,i}^{1/2}\lambda_{2,j}^{1/2}}.\\
    &=\frac{
        \dotp{e_{1,i}}{\Kscr_{12}e_{2,j}}
    }{
        \lambda_{1,i}^{1/2}\lambda_{2,j}^{1/2}
    }\\
    &=\frac{
        \dotp{\Rscr_{12}\Kscr_2^{1/2}e_{2,j}}{\Kscr_{1}^{1/2}e_{1,i}}
    }{
        \lambda_{1,i}^{1/2}\lambda_{2,j}^{1/2}        
    }
    \\
    &=\dotp{e_{1,i}}{\Rscr_{12}e_{2,j}}.
\end{align*}
Since $\{\tilde{e}_{m,j}\}_{j\in\NN}$ forms a CONS for $\GG_{m}$ and $\{e_{m,j}\}_{j\in\NN}$ forms a CONS for $\HH_m$ for $m=1,2$, we can write
\[
\Cscr_{12}=\sum_{i,j=1}^\infty\dotp{\tilde{e}_{1,i}}{\Cscr_{12}\tilde{e}_{2,j}}_{\GG_1}\tilde{e}_{1,i}\otimes\tilde{e}_{2,j},\quad 
\Rscr_{12} = \sum_{i,j=1}^\infty
\dotp{e_{1,i}}{\Rscr_{12}e_{2,j}}e_{1,i}\otimes e_{2,j}.
\]
Under the assumption of compactness, both $\Cscr_{12}$ and $\Rscr_{12}$ admit a singular system. Then,~\eqref{eq:RCsvd} is the direct consequence of~\eqref{eq:RequalC}. 
\end{proof}
\subsection{Proof of Theorem~\ref{theorem:cca2svd}}
 First, we want to show the existence of $\Cscr_{12}:\GG_{2}\rightarrow\GG_{1}$. Lemma~\ref{lemma:existence_c} tells that there exists a $\Cscr_{12}\in\mathfrak{B}(\GG_{2}, \GG_{1})$ satisfying $\dotp{f}{\Cscr_{12}g}_{\GG_{1}}=\Cov(\dotp{\bar\chi_1}{f}\dotp{\bar\chi_2}{g})$ for all $f\in\GG_{1}$ and $g\in\GG_{2}$. 

Since $\{\tilde{e}_{1,j}\}_{j\in\NN}$ forms a CONS for $\GG_{1}$ and $\{\tilde{e}_{2,j}\}_{j\in\NN}$ forms a CONS for $\GG_{2}$, we can write
\[
\Cscr_{12} 
= 
\sum_{i,j=1}^\infty
\dotp{\tilde{e}_{1,i}}{\Cscr_{12}\tilde{e}_{2,j}}_{\GG_{1}}
\tilde{e}_{1,i}\otimes \tilde{e}_{2,j}
\]

Under the assumption that $\Cscr_{12}$ is compact, then by Theorem 4.3.1 in \citep{hsing2015theoretical}, there exists a singular system $\{(\gamma_j,f_{1,j},f_{2,j})\}_{j\in\NN}$. Consider $j=1$ and write
\[
\gamma_1 = \dotp{f_{1,1}}{\Cscr_{12}f_{1,2}}_{\GG(\Kscr{1})} =
\Cov(
\dotp{\chi_1}{f_{1,1}}
\dotp{\chi_2}{f_{1,2}}
).
\]
Therefore, we can write
\[
\gamma_1 = \max{f_1\in\GG_{1},\; f_2\in\GG_{2}} \Cov(
\dotp{\chi_1}{f_{1,1}}
\dotp{\chi_2}{f_{1,2}}
).
\]
Recall that
\begin{align*}
    \rho_1^\star &= \frac{
        \Cov(
        \dotp{\chi_1}{g_{1,j}^\star}
        \dotp{\chi_2}{g_{2,j}^\star}
        )
    }{
        \Var^{1/2}(\dotp{\chi_1}{g_{1,1}^\star})
        \Var^{1/2}(\dotp{\chi_2}{g_{2,1}^\star})
    }\\
    &= \frac{
        \Cov(
        \dotp{\chi_1}{g_{1,1}^\star}
        \dotp{\chi_2}{g_{2,1}^\star}
        )
    }{
        \norm{g_{1,1}^\star}_{\GG_{1}}
        \norm{g_{2,1}^\star}_{\GG_{2}}
    }\\
    &= \Cov\rbr{
    \left\langle
        \chi_1,
        \frac{g_{1,1}^\star}{\norm{g_{1,1}^\star}_{\GG_{1}}}
    \right\rangle
    \left\langle
        \chi_2,
        \frac{g_{2,1}^\star}{\norm{g_{2,1}^\star}_{\GG_{2}}}
    \right\rangle
    }
\end{align*}
Since we know that $g_{1,1}^\star$ and $g_{2,1}^\star$ maximize~\eqref{eq:correlation_p} by definition. Hence one pair of solution is $(\rho_1^\star,
g_{1,1}^\star/\norm{g_{1,1}^\star}_{\GG_{1}},
g_{2,1}^\star/\norm{g_{2,1}^\star}_{\GG_{2}}
)=(\gamma_1, f_1,f_2)$. 
Note that, by definition of singular system, we have
\[
\dotp{f_{1,j}}{f_{1,j'}}_{\GG_{1}} = 0,\quad \dotp{f_{2,j}}{f_{2,j'}}_{\GG_{2}}=0,\quad j\neq j'.
\]
This implies that for $m=1,2$:
\begin{align*}
\dotp{f_{m,j}}{f_{m,j'}}_{\GG_{m}}
&=
\sum_{i=1}^\infty\lambda_{m,i}\dotp{f_{m,j}}{e_{m,i}}\dotp{f_{m,j}}{e_{m,i}}\\
&=
\dotp{\Kscr_{m}f_{m,j}}{f_{m,j'}}\\
&=
\Cov(\dotp{\bar\chi_i}{f_{m,j}}
\dotp{\bar\chi_i}{f_{m,j'}}
)=0,
\end{align*}
which satisfies the constraint in~\eqref{eq:ccaproblem}. Therefore the general result follows similarly. 

\subsection{Proof of Theorem~\ref{theorem:iniA}}
%$\norm{\hat\Ab_1^k-\Ab_1^{k\star}}$
%The distance of $\norm{\hat\Ab_2^k-\Ab_2^{k\star}}$ can be obtained in the same way, and hence we only discuss one side. 
Given  $\ell\in\NN$, assume that $\hat g_{1,\ell}$ converges to $\bar g_{1,\ell}$. We denote the corresponding $\bar\Ab_1^{k}$. Apply triangle inequality, we have
\[
\norm{\hat\Ab_1^k-\Ab_1^{k\star}}_F^2\leq 
2\rbr{
\norm{\hat\Ab_1^k-\bar\Ab_1^{k}}_F^2
+
\norm{\bar\Ab_1^k-\Ab_1^{k\star}}_F^2}.
\]
We bound the two terms on the left hand side by the following lemmas:

\begin{lemma}\label{lemma:method2_2}
    Under Assumption~\ref{assumption1} and 
    define $\|\Cscr_{12}^{k_1,k_2}-\Cscr_{12}\|_{HS}:=\delta_{k_1,k_2}$. Then, there exist a  constant $C$ depending on the singular values of $\Cscr_{12}$ such that
    \[
    \norm{\bar\Ab_1^k-\Ab_1^{k\star}}_F^2
    =
    C\lambda_{1,k_1}^{-1}k\delta_{k_1,k_2}^2.
    \]
\end{lemma}

\begin{lemma}\label{lemma:method2}
    Under Assumption~\ref{assumption1}
    and define
    \begin{equation}\label{eq:defzeta}
    \zeta_{m,j}=\frac{1}{2}\inf_{s\neq j}|\lambda_{m,j}-\lambda_{m,s}|,\quad \zeta_m^{k} = \min_{j\leq k}\zeta_{m,j},\quad i=1,2.
    \end{equation}
    Assume that 
    $\varepsilon_N:=\max\{
    \norm{\hat\Kscr_1-\Kscr_1},
    \norm{\hat\Kscr_{12}-\Kscr_{12}},
    \norm{\hat\Kscr_2-\Kscr_2}
    \}$ such that 
    \begin{equation}\label{eq:condition_a}
    \varepsilon_N
    <
    \min_{m=1,2}\zeta_m^{k_m}.
    \end{equation}
    Then, there exists constants $C_1, C_2$ such that
    \begin{multline*}
    \norm{\hat\Ab_1^{k} - \bar\Ab_1^{k}}_F^2
    = 
    C_1\cbr{
    (\lambda^{-1}_{1,k_1}\vee 1)
    (\lambda_{1,k_1}^{-3}\vee \lambda_{2,k_2}^{-3})
    (k\vee k_1)
    \varepsilon_N^2}\\
    +
    C_2\cbr{\lambda^{-1}_{1,k_1}k
    ((1\vee\lambda_{1,k_1}^{-1}k_1)k_1
    (\zeta_1^{k_1})^{-2}\vee \lambda_{2,k_2}^{-1}k_2^2(\zeta_2^{k_2})^{-2})
    \varepsilon_N^2}.
    \end{multline*}
    
\end{lemma}
Given that $\varepsilon_N$ is some random quantity, we want to find the probability that condition~\eqref{eq:condition_a} hold. We can apply Lemma~\ref{lemma:Kscr_sample bound}--\ref{lemma:HSop_tail} and obtain the followings. Let $\zeta=\min_{m=1,2}\zeta_{m}^{k_m}$. 
If $\SCthree$, then
\begin{align*}
     \hsnorm{\hat\Kscr_{1}-\Kscr_{1}} \geq \norm{\hat\Kscr_{1}-\Kscr_{1}}\geq \zeta,
\end{align*}
with probability smaller than $\delta$. We can bound $\norm{\hat\Kscr_2-\Kscr_2}$ and $\norm{\hat\Kscr_{12}-\Kscr_{12}}$ using the same approach. Taking the union bound we can conclude that the event
\[
\Ecal(\zeta)=\{\varepsilon_N<\zeta\}
\]
happens with probability at least $1-3\delta$. Then, on the event of $\Ecal(\zeta)$, we can apply Lemma~\ref{lemma:method2}.

\subsection{Proofs of Lemma~\ref{lemma:method2_2}--\ref{lemma:method2}}
\begin{proof}[Proof of Lemma~\ref{lemma:method2_2}]
Recall that
$a_{1,ij}^{k\star}
=\dotp{g_{1,i}^\star}{{e}_{1,j}}
=u_{i,j}/\lambda_{1,j}^{1/2}$ for $i=1,\ldots, k$ and $j=1,\ldots,k_1$.
Define ${g}_{1,i}^{k_1\star}=\sum_{k=1}^{k_1}\dotp{g_{1,i}^\star}{\tilde{e}_{1,j}}_{\GG_1}\tilde{e}_{1,j}$ and ${g}_{1,i}^{k_1+\star}=\sum_{k_1}^{\infty}\dotp{g_{1,i}^\star}{\tilde{e}_{1,j}}_{\GG_1}\tilde{e}_{1,j}$. Let $\{(\bar\rho_j,\bar g_{1,i}^{k_1}, \bar g_{2,i}^{k_2})\}$ be the singular system of $\Cscr_{12}^{k_1,k_2}$ such that $\bar g_{1,i}^{k_1}=\sum_{j=1}^{k_1}\dotp{\bar g_{1,i}^{k_1}}{\tilde{e}_{1,j}}_{\GG_1}\tilde{e}_{1,j}
=\sum_{j=1}^{k_1}\bar u_{i,j}\tilde{e}_{1,j}$ and $\bar a_{1,ij}^{k}=\dotp{\bar g_{1,i}^{k_1}}{{e}_{1,j}}$ for $i=1,\ldots,k$ and $j=1,\ldots,k_1$.

Write
\begin{align*}
    \norm{\bar\Ab_1^k-\Ab_1^{k\star}}_F^2
    =
    \norm{(\bar U^k - U^{k\star})^\top\Sigma^{-1/2}}_F^2
    &\leq \lambda_{1,k_1}^{-1}
    \norm{\bar U^k- U^{k\star}}_F^2\\
    &\leq \lambda_{1,k_1}^{-1}\sum_{i=1}^k\norm{\bar g_{1,i}^{k_1}-g_{1,i}^{k_1\star}}_{\GG_1}^2\\
    &\leq
    \lambda_{1,k_1}^{-1}
    \sum_{i=1}^k(
    \norm{
        \bar g_{1,i}^{k_1}
        -
        g_{1,i}^{k_1\star}
    }_{\GG_1}^2
    +
    \norm{g_{1,i}^{k_1+\star}}_{\GG_1}^2
    )\\
    &= \lambda_{1,k_1}^{-1}\sum_{i=1}^k
    \norm{\bar g_{1,i}^{k_1} - g_{1,i}^{\star}}_{\GG_1}^2.
\end{align*}

Observe that for $i=1,\ldots,k$, $g_{1,i}^{k_1}$ is the left singular function of $\Cscr_{12}^{k_1,k_2}$ and $g_{1,i}$ is the left singular function of $\Cscr_{12}$ and hence we can apply Theorem 5.2.2 in~\citet{hsing2015theoretical}. Define $\Tscr = \Cscr_{12}^{k_1,k_2}-\Cscr_{12}$:
\begin{align}
    \norm{\bar g_{1,i}^{k_1} - g_{1,i}^{\star}}_{\GG_1}^2
    &=\bignorm{\sum_{i\neq j}\frac{
        \rho_j
        \dotp{g_{1,i}^{\star}}{\Tscr g_{2,j}^\star}_{\GG_1}
        -
        \rho_i
        \dotp{g_{1,j}^{\star}}{\Tscr{g}_{2,i}^\star}_{\GG_1}
    }{\rho_j^2-\rho_i^2}
    g_{1,i}^{\star}
    }_{\GG_1}^2\notag\\
    &\leq 
    \frac{2\rho_1}{\min_{i\neq j}\rho_j^2-\rho_i^2}
    \rbr{
        \sum_{i\neq j}\dotp{g_{1,i}^\star}{\Tscr g_{2,j}^\star}_{\GG_1}^2
        +
        \sum_{i\neq j}\dotp{g_{1,j}^\star}{\Tscr g_{2,i}^\star}_{\GG_1}^2
    }\notag\\
    &\leq
    \frac{2\rho_1}{\min_{i\neq j}\rho_j^2-\rho_i^2}
    \rbr{
        \norm{\Tscr^*g_{1,i}^\star}_{\GG_2}^2 + \norm{\Tscr g_{2,i}^\star}_{\GG_1}^2 
    } = C(\norm{\Tscr}_2^2),\label{eq:barA_Astar}
\end{align}
\marginnote{The canonical correlation should be distinct. Otherwise, the solution is not identifiable.}
for some constant $C\geq 0$.
Plugging the above result back~\eqref{eq:barA_Astar}, we obtain that
\[
\norm{\bar\Ab_1^k-\Ab_1^{k\star}}_F^2=C(\lambda_{1,k_1}^{-1} k\delta_{k_1,k2}^2).
\]
\end{proof}
\begin{proof}[Proof of Lemma~\ref{lemma:method2}]
Define
\[\hat\Sigma = \begin{pmatrix}
\hat\lambda_{1,1}&0&\ldots&0\\
0&\hat\lambda_{1,2}&\ldots&0\\
&&\ddots&\\
0&0&\ldots&\hat\lambda_{1,k_1}\\
\end{pmatrix},\quad 
\Sigma = \begin{pmatrix}
\lambda_{1,1}&0&\ldots&0\\
0&\lambda_{1,2}&\ldots&0\\
&&\ddots&\\
0&0&\ldots&\lambda_{1,k_1}\\
\end{pmatrix}.
\]
Therefore, by triangle inequality, we can write 
\begin{align*}
    \norm{\hat\Ab_1^k - \bar\Ab_1^{k}}_F&=
    \norm{\hat{U}^{k\top}\hat\Sigma^{-1/2}-\bar U^{k\top}\Sigma^{-1/2}}_F\\
    &\leq 
    \norm{\hat{U}^{k\top}(\hat\Sigma^{-1/2}-\Sigma^{-1/2})}_F
    +
    \norm{(\hat{U}^{k\top}-\bar U^{k\top})\Sigma^{-1/2}}_F.
\end{align*}
Write
\begin{align}\label{eq:3}
    \norm{\hat{U}^{k\top}(\hat\Sigma^{-1/2}-\Sigma^{-1/2})}_F^2\leq 
    \sum_{j=1}^{k_1}|\hat\lambda_{1,j}^{-1/2}-\lambda_{1,j}^{-1/2}|^2=o_p(k_1\lambda_{1,k_1}^{-3}\varepsilon_N^2),
\end{align}
where the last equality follows from~\eqref{eq:inv}.
For the second term, write
\begin{align*}
\norm{(\hat{U}^{k\top}-\bar U^{k\top})\Sigma^{-1/2}}_F^2
&\leq \lambda_{1,k_1}^{-1}\sum_{i=1}^k\norm{\hat u_{i}-\bar{u}_{i}}_2^2\\
&=
\lambda_{1,k_1}^{-1}\sum_{i=1}^k
\bignorm{\sum_{j=1}^{k_1}
\hat u_{i,j}e_{1,j}
-
\sum_{j=1}^{k_1}\bar u_{i,j}e_{1,j}}_{\HH_1}^2\\
&=
\lambda_{1,k_1}^{-1}\sum_{i=1}^k
\bignorm{
\sum_{j=1}^{k_1}\hat u_{i,j}(e_{1,j}-\hat{e}_{1,j})
+\sum_{j=1}^{k_1}\hat u_{i,j}\hat{e}_{1,j}
-\sum_{j=1}^{k_1}\bar u_{i,j}e_{1,j}
}_{\HH_1}^2.\\
\intertext{For $i=1,\ldots,k$, define $
\hat{g}_{1,i}^{k_1\sharp}:=
\sum_{j=1}^{k_1}
\hat u_{i,j}
\hat e_{1,j}$, which is the left singular function of $\hat\Rscr_{12}^{k_1,k_2}=(\hat{\Kscr}_1^{k_1})^{-1/2}\hat\Kscr_{12}(\hat{\Kscr}_2^{k_2})^{-1/2}$ by Lemma~\ref{lemma:RC_svd}. Similarly, for $i=1,\ldots,k$, 
define $
\bar{g}_{1,i}^{k_1\sharp}:=
\sum_{j=1}^{k_1}
\bar u_{i,j}
 e_{1,j}$,
 which is the left singular function of $\Rscr_{12}^{k_1,k_2}=(\Kscr_1^{k_1})^{-1/2}\Kscr_{12}(\Kscr_2^{k_2})^{-1/2}$. Then, we can bound the above display as
} 
&\leq
2\lambda_{1,k_1}^{-1}\sum_{i=1}^k
\cbr{\norm{
    \sum_{j=1}^{k_1}
        \hat u_{i,j}(e_{1,j}-\hat{e}_{1,j})}_{\HH_1}^2
    +
    \norm{\hat g_{1,i}^{k_1} - \bar g_{1,i}^{k_1}}_{\HH_1}^2
}\\
&\leq  
2\lambda_{1k_1}^{-1} \rbr{
kk_1\max_{i\leq k_1}\norm{e_i-\hat{e}_{i}}_{\HH_1}^2
+
\sum_{j=1}^k
\norm{\hat g_{1,i}^{k_1} - \bar g_{1,i}^{k_1}}_{\HH_1}^2
}.
\end{align*}
Apply Theorem 5.1.8 in \citep{hsing2015theoretical} to the first term and Lemma~\ref{lemma:r12_difference} to the second term, we can conclude that
\begin{multline}\label{eq:4}
\norm{(\hat U^{k\top}-\bar U^{k\top})\Sigma^{-1/2}}_F^2
=O_p(kk_1(\zeta_1^{k_1})^{-2}\varepsilon_N^2\lambda_{1,k_1}^{-1})
+
o_p(k\varepsilon_N^2\lambda^{-1}_{1,k_1}(\lambda_{1k_1}^{-3}\vee \lambda_{2k_2}^{-3}))\\
+
O_p(k\varepsilon_N^2\lambda^{-1}_{1,k_1}\{(\lambda_{1,k_2}^{-1}k_1^2(\zeta_1^{k_1})^{-2}\vee \lambda_{2,k_2}^{-1}k_2^2(\zeta_2^{k_2})^{-2})\})
.
\end{multline}
Combining~\eqref{eq:3}--\eqref{eq:4}, we complete the proof.
\end{proof}
