# Supplementary material for: Latent Multimodal Functional Graphical Model Estimation
Source: arXiv:2210.17237 source file (2023-10-01)
Supplement: Supplementary file 3 [file 6_generalized_CCA.tex]

\section{Generalized Canonical Correlation problems}\label{sec:GneralCCA}
\[
\Jb(\gb)=\min_{\zb,\rb}\frac{1}{M}\sum_{m=1}^M\norm{\zb-r_m^{(\ell)}\yb^{m, (\ell)}}_2^2,
\]
where $\rb^{(\ell)}=(r_1^{(\ell)},\ldots,r_M^{(\ell)})$ is the weight vector and $\norm{\zb}_2^2=\norm{\rb^{(\ell)}}_2^2=M$ to avoid trivial solutions. The above cost function can be reformulated as an eigendecomposition problem. 

In the functional setting, we use the similar approach discussed in Section~\ref{sec:reasoning}. However, we do not restrict the basis functions to be the set of the eigenfunctions of the covariance operators. Therefore we can pick $f^{(\ell)}=\varphi^0_\ell$ and we define
\[
    \Ycal^{m,n,(\ell)}
    =
    \dotp{
        \Ascr_m\chi^{m,n}}{f^{(\ell)}
    }
    f^{(\ell)},\quad 
        \Ycal^{m,k_m,n,(\ell)}
    =
    \dotp{
        \Ascr_m\chi^{m,k_m,n}}{f^{(\ell)}
    }
    f^{(\ell)},
\]
where $\chi^{m,k_m,n}$ is the truncated version of $\chi^{m,n}$. and
\[
    g^{m,(\ell)}
    =
    \sum_{\ell'=1}^{\infty}\dotp{ \Ascr_m^*f^{(\ell)}}{\varphi_{\ell'}^m}\varphi_{\ell'}^m
    ,\quad
    g^{m,k_m,(\ell)}
    = \sum_{\ell'=1}^{k_m}\dotp{ \Ascr_m^*f^{(\ell)}}{\varphi_{\ell'}^m}\varphi_{\ell'}^m.
\]
Stacking the samples $\nseq$ together, we define
\[
\Ycal^{m,(\ell)}
=
    \begin{pmatrix}
        \Ycal^{m,1,(\ell)}\\
        \vdots\\
        \Ycal^{m,N,(\ell)}
    \end{pmatrix}\in\HH_m^N,\quad\mseq,\quad
\Ycal^{m,k_m,(\ell)}
=
    \begin{pmatrix}
        \Ycal^{m,k_m,1,(\ell)}\\
        \vdots\\
        \Ycal^{m,k_m,N,(\ell)}
    \end{pmatrix}\in\HH_m^N,\quad\mseq,
\]
and 
$
\Gcal^{(\ell)}
=
\{ g^{1,(\ell)},\ldots, g^{M,(\ell)}\}$. Then, we define the objective function to be
\begin{equation}\label{eq:dirobj}
\Jb(\Gcal^{(\ell)})
=
\min_{\chi^z,\rb^{(\ell)}}
\frac{1}{MN}\sum_{m=1}^M
\norm{\chi^z - r_m^{(\ell)}\Ycal^{m,(\ell)}}_{\HH_0^N}^2,
\end{equation}
where we restrict $\norm{\Ycal^{m,(\ell)}}_{\HH_0^N}^2=N$ for $\mseq$ and $\norm{\rb^{(\ell)}}_2^2=M$.

To find the Fr\'echet derivative of $\Jb(\Gcal^{(\ell)})$ with respect to $\chi^z$, we can write
\begin{align*}
    \lim_{{t\rightarrow 0}}
    \frac{1}{MN}\sum_{m=1}^M&
    \frac{
        {\norm{
            (\chi^z+t\Delta) 
            - 
            r_m^{(\ell)}\Ycal^{m,(\ell)}
        }_{\HH_0^N}^2
        -
        \norm{
            \chi^z 
            - 
            r_m^{(\ell)}\Ycal^{m,(\ell)}
        }_{\HH_0^N}^2}}{
            \norm{t\Delta}_{\HH_0^N}
        }\\
    &=
        \frac{2}{MN}\sum_{m=1}^M
        \left\langle{
            \frac{
                \Delta}{
                \norm{\Delta}_{\HH_0^N}
            }},{
            \chi^z
            -
            r_m^{(\ell)\Ycal^{m,(\ell)}}
        }\right\rangle_{\HH_0^N}.\\
\end{align*}
This implies that
\begin{align*}
D(\Delta)=\frac{2}{MN}\sum_{m=1}^M
        \left\langle
        \Delta
        ,{
            \chi^z
            -
            r_m^{(\ell)\Ycal^{m,(\ell)}}
        }\right\rangle_{\HH_0^N}
        =\frac{2}{N}\sum_{n=1}^N\sum_{\ell'=1}^\infty\cbr{
        \left\langle
                \Delta_n
            ,
            \varphi_{\ell'}^0
        \right\rangle
        \left\langle
            \chi^z_n
            -
            r_m^{(\ell)\Ycal^{m,n,(\ell)}}
            ,
            \varphi_{\ell'}^0
        \right\rangle
        }.
\end{align*}
To obtain $D(\Delta)=0$ for all $\Delta\in\HH_0^N$, one solution is 
\begin{align}\label{eq:optimalz}
    \chi^z = \frac{1}{M}\sum_{m=1}r_m^{(\ell)}\Ycal^{m,(\ell)}.
\end{align}
Then, plug~\eqref{eq:optimalz} back to ~\eqref{eq:dirobj}, we have
\[
\Jb(\Gcal^{(\ell)})
=
\min_{\rb^{(\ell)}}
\frac{1}{MN}\sum_{m=1}^M
\norm{r_m^{(\ell)}\Ycal^{m,(\ell)}}_{\HH_0^N}^2
-
\frac{1}{N}\bignorm{
\frac{1}{M}\sum_{m=1}^M
r_m^{(\ell)}\Ycal^{m,(\ell)}
}_{\HH_0^N}^2.
\]
Although this problem is a joint optimization of $\Gcal^{(\ell)}$ and $\rb^{(k)}$, which is nonconvex, we can reformulate the problem into a eigendecomposition problem and hence unique optimal solution can be obtained (as long as eigenvalues of the covariance are distinct or maybe some eigengaps).

Now because of many many reasons, we consider finding the optimal solution of the truncated $\Jb(\Gcal^{(\ell)})$:
\begin{equation}\label{eq:dirobj2}
\Jb(\Gcal^{(\ell)})
=
\min_{\chi^z,\rb^{(\ell)}}
\frac{1}{MN}\sum_{m=1}^M
\norm{\chi^z - r_m^{(\ell)}\Ycal^{m,k_m,(\ell)}}_{\HH_0^N}^2
\end{equation}
Repeat the above steps, we have
\[
    \chi^z
    =
        \frac{1}{M}\sum_{m=1}^M
        r_m^{(\ell)}
        \Ycal^{m,k_m,(\ell)},
\]
and define
\[
\yb^{m,k_m,n,(\ell)}
=\dotp{\Ycal^{m,k_m,n,(\ell)}}{f^{(\ell)}}=\xb^{m,k_m,n\top}\ab_m^{(\ell)}
,\quad\mseq,\nseq,
\]
and 
\begin{align*}
&\yb^{m,k_m,(\ell)}
=
\begin{pmatrix}
\yb^{m,k_m,1,(\ell)}\\
\vdots\\
\yb^{m,k_m,N,(\ell)}
\end{pmatrix}
=\Xb^{m,k_m\top}\ab^{m,k_m,(\ell)}
\in\RR^N;\\
&\Yb^{(\ell)}=\begin{pmatrix}
\yb^{1,k_1,(\ell)}&\ldots&\yb^{M,k_M,(\ell)}
\end{pmatrix}\in\RR^{N\times M}.
\end{align*}
Therefore, we can write
\[
\begin{pmatrix}
\dotp{\chi^z_1}{f^{(\ell)}}_{\HH_0}\\
\vdots\\
\dotp{\chi^z_N}{f^{(\ell)}}_{\HH_0}
\end{pmatrix}
 =\frac{1}{M}\Yb^{(\ell)}\rb^{\ell}\in\RR^{N}. 
\]
Hence we can present~\eqref{eq:dirobj2} as
\begin{align*}
    \Jb(\Gcal^{(\ell)})
    &=
        \min_{\rb^{(\ell)}}
        \frac{1}{MN}\sum_{m=1}^M
        \norm{ 
            r_m^{(\ell)}\Ycal^{m,k_m,(\ell)}
        }_{\HH_0^N}^2
        -
        \frac{1}{NM^2}
        \rb^{(\ell) \top}
        \Yb^{(\ell) \top}
        \Yb^{(\ell)}
        \rb^{(\ell)}\\
    &=  \min_{\rb^{(\ell)}}
        1
        -
        \frac{1}{NM^2}
        \rb^{(\ell) \top}
        \Yb^{(\ell) \top}
        \Yb^{(\ell)}
        \rb^{(\ell)},
\end{align*}
which is an eigendecomposition problem.

Next, we write the eigendecomposition as 
\[
    \Xb^{m,k_m\top}=\Ub^{m}\Sigmab^m\Vb^{m\top},\quad\mseq,
\]
and hence 
\[
    r_m^{(\ell)}\yb^{m,k_m,(\ell)}=r_m^{(\ell)}\Ub^{m}\{\Sigmab^m\Vb^{m\top}\ab^{m,k_m,(\ell)}\}=:\Ub^{m}\tilde\ab^{m,k_m,(\ell)}.
\]
Let 
$
\tilde\ab^{(\ell)}
    =
    (\tilde\ab^{1,k_1,(\ell)\top},\ldots,\tilde\ab^{M,k_M,(\ell)\top})^\top
$
and
$\Ub = (\Ub^{1},\ldots,\Ub^{M})$
, then we can write
\[
\frac{1}{NM^2}
\rb^{(\ell)\top}
\Yb^{(\ell)\top}
\Yb^{(\ell)}
\rb^{(\ell)}
=
    \frac{1}{NM^2}
    \tilde\ab^{(\ell)\top}
    \Ub^\top
    \Ub
    \tilde\ab^{(\ell)}.
\]
The above display is maximized if we take $\tilde\ab^{(\ell)}$ be the $\ell$-th eigenvector of $\Ub^\top\Ub$ and $\tilde\ab^{(\ell)}$ is orthogonal to $\tilde\ab^{(\ell')}$ for $\ell'=1,\ldots, \ell-1$. After rescaling, we can get $\{(\ab^{m,k_m,(\ell),r_m})\}_{m=1}^M$.
Given $m$, this method does not guarantee that $\ab^{m,k_m,(\ell)}\perp\ab^{m,k_m,(\ell')}$ for $\ell'\neq\ell$. Therefore, we can not say anything about the row structure of $\hat\Ab_m^k$. But any pair of rows in $(\hat\Ab_1^k,\ldots,\hat\Ab_m^k)$ is orthogonal.

\begin{algorithm}\label{alg:cca}
\SetAlgoLined
\KwIn{$\{\Xb^{m,k_m}\}_{\mseq}$}
\KwResult{$\{\hat\Ab_m^k\}_{\mseq}$, ${\rb^{(\ell)}}_{\ell=1,\ldots,k}$}
\For{$\mseq$}{
    compute singular value decomposition\;
    $(\Ub^m,\Sigmab^m,\Vb^{m\top})\leftarrow \text{SVD}(\Xb^{m,k_m\top})$\;
}
\For{$\ell=1,\ldots,k$}{
 $\tilde\ab^{(\ell)}\leftarrow\ell\text{-th eigenvector of } \Ub^\top\Ub$\;
 \For{$\mseq$}{
    $\hat\Ab_{m,\ell\cdot}^{k}
    \leftarrow
    \frac{
        \sqrt{N}}{
        \norm{\tilde\ab^{m,k_m,(\ell)
    }}_2}
    \cbr{(\Sigmab^{m})^{-1}
    \Vb^{m\top}
    \tilde\ab^{m,k_m,(\ell)}}^\top$\;
 }
 $\rb^{(\ell)}
     =
     \frac{\sqrt{M}}{
        \sum_{m=1}^M\norm{\tilde\ab^{m,k_m,(\ell)
        }}_2
    }(\norm{\tilde\ab^{1,k_1,(\ell)
        }}_2,\ldots,\norm{\tilde\ab^{M,k_M,(\ell)
        }}_2)
$\;
 }
 
 \caption{Generalized Canonical Correlation Analysis}
\end{algorithm}
